# Supplementary material for: A Time-Reversal Control Synthesis for Steering the State of Stochastic Systems
Source: arXiv:2504.00238 source file (2025-09-09)
Supplement: Supplementary file 1 [file appendix.tex]

% To obtain $p(t,x)$, we only need to find the mean and covariance of $Z_t$. Taking expectations on both sides of \eqref{eq:Z-lin}
% \begin{equation}\label{eq:mean-dyn}
%     \ud \Expect [Z_t] = -A \Expect[Z_t]\ud t, ~~ \Expect[Z_0] = x_f
% \end{equation}
% Let $m_t$ denote the mean of $Z_t$, we can obtain 
% \begin{equation}
%     m_t = e^{-At}x_f
% \end{equation}
% Let $\Sigma_t$ denote the covariance of $Z_t$, and $\Sigma_t = \Expect [Z_t Z_t^\top] - \Expect[Z_t]\Expect[Z_t]^\top$.
% \begin{align}
%     \ud \Sigma_t = \Expect[\ud Z_t Z_t^\top + Z_t \ud Z_t^\top + \ud Z_t \ud Z_t^\top] - \nonumber \\
%     \ud \Expect[Z_t] \Expect[Z_t]^\top - \Expect[Z_t] \ud \Expect[Z_t]^\top
% \end{align}
% \begin{align}\label{eq:cov-dyn}
%     \frac{\ud}{\ud t} \Sigma_t = -A \Sigma_t - \Sigma_t A^\top + \epsilon^2 B B^\top, ~~ \Sigma_0 = 0
% \end{align}
% The solution for $\Sigma_t$ is
% \begin{equation}
%     \Sigma_t =  \epsilon^2 \int_0^t e^{-A(t-s)}BB^\top e^{-A^\top(t-s)}\ud s
% \end{equation}
